# Supplementary material for: High-Order Topological Phase Diagram Revealed by Anomalous Nernst Effect in Janus ScClI Monolayer
Source: arXiv:2308.07550 source file (2024-01-30)
Supplement: Supplementary file 1 [file SM.pdf]

# Supplementary materials

## High-Order Topological Phase Diagram Revealed by Anomalous Nernst Effect in Janus ScClI Monolayer

Ning-Jing Yang[1,2] and Jian-Min Zhang[1,2*]

*1 Fujian Provincial Key Laboratory of Quantum Manipulation and New Energy Materials, College of Physics and Energy, Fujian Normal University, Fuzhou 350117, China and*

*2 Fujian Provincial Collaborative Innovation Center for Advanced High-Field Superconducting Materials and Engineering, Fuzhou, 350117, China*

(Dated: December 5, 2023)

### I. ORBITAL VERIFICATION OF HIGH ORDER TOPOLOGY

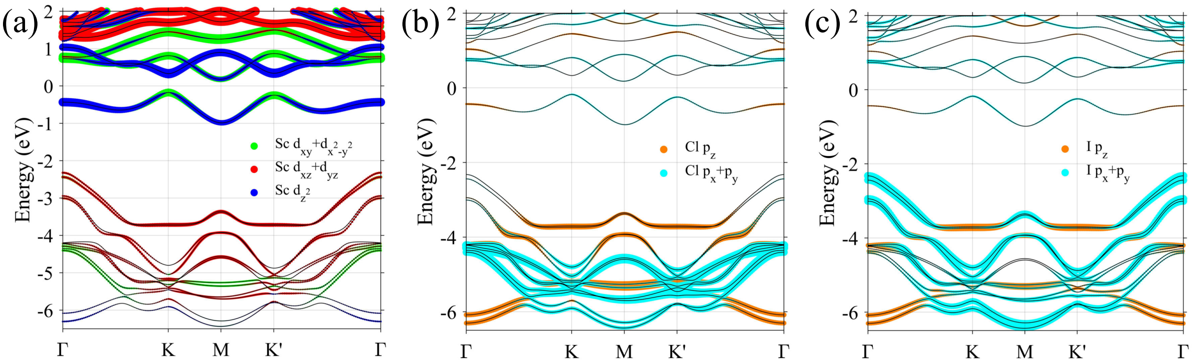


FIG. S1: The fatbands of individual atomic projected orbitals are shown in (a, b, c), respectively.

*Corresponding author:`jmzhang@fjnu.edu.cn`

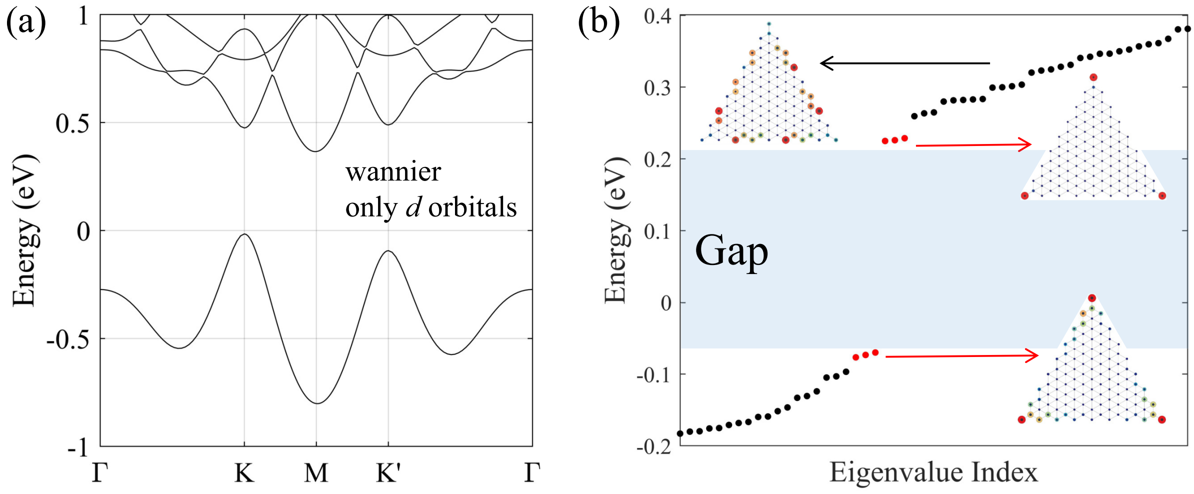


FIG. S2: (a) Energy band structure of the $d$-orbitals in ScClI. (b) Energy spectrum of a triangular quantum dot based on the tight-binding model for $d$-orbitals.

If we focus solely on the $d$-orbital contribution from Sc atoms, the tight-binding model includes a total of $2 \cdot 5$ orbitals, where the factor of 2 represents the spin index. Regrettably, the presence of only one occupied band below the Fermi level results in the corner charge $Q_c^{(3)}$ being equal to zero. Fig. S2(a) displays the energy band consisting exclusively of $d$ orbitals, as obtained from the Wannier bases. At this point, the tight-binding model is a single lattice-dot model. In the energy spectrum of its triangular quantum dots, there is a distinct band gap with no topologically protected corner states near the Fermi energy level, as shown in Fig. S2(b). Although corner-localized states appears, it is characterized as more defect-induced and non-topological.

## II. ROBUSTNESS OF HIGH-ORDER TOPOLOGY

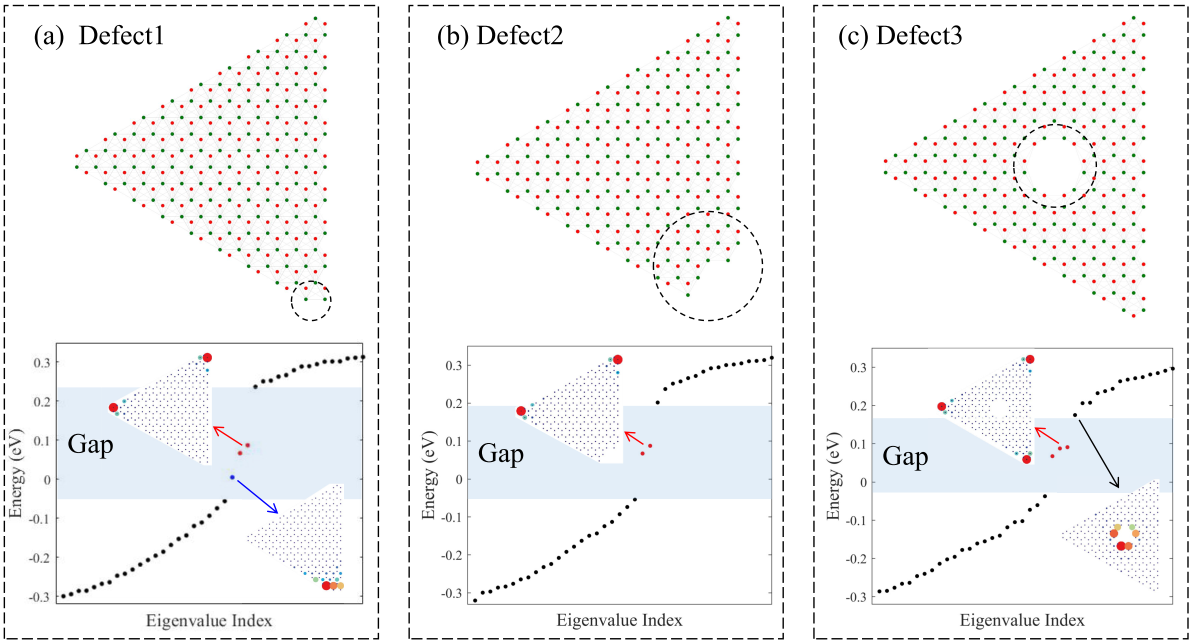


FIG. S3: Three defect structures and their corresponding energy spectra.

Intrinsic corner states are highly robust, due to being symmetry-protected. For this protection, topological states are generally resistant to defects. In this section, we do three defect treatments for the ScClI triangular quantum dot, as shown in Fig. S3. However, when we dig out one atom, the corner state at that position degenerates toward the edge state and its eigenvalue shifts downward. While the other two corner states are not affected. In Fig. S3(b), we expand the defect region and the band gap still maintains the eigenvalues of the two corner states. In Fig. S3(c), we dig out a circular defect in the center region, the higher-order topological corner states are not affected. For general systems, defect states often appear at the Fermi energy, so called zero-energy states, and affect other states. In our system, the higher order topological angular states are robust enough that they are not disturbed in any way.

## III. MAGNETIC VALLEY COUPLING EFFECTS AND OTHER DFT RESULTS

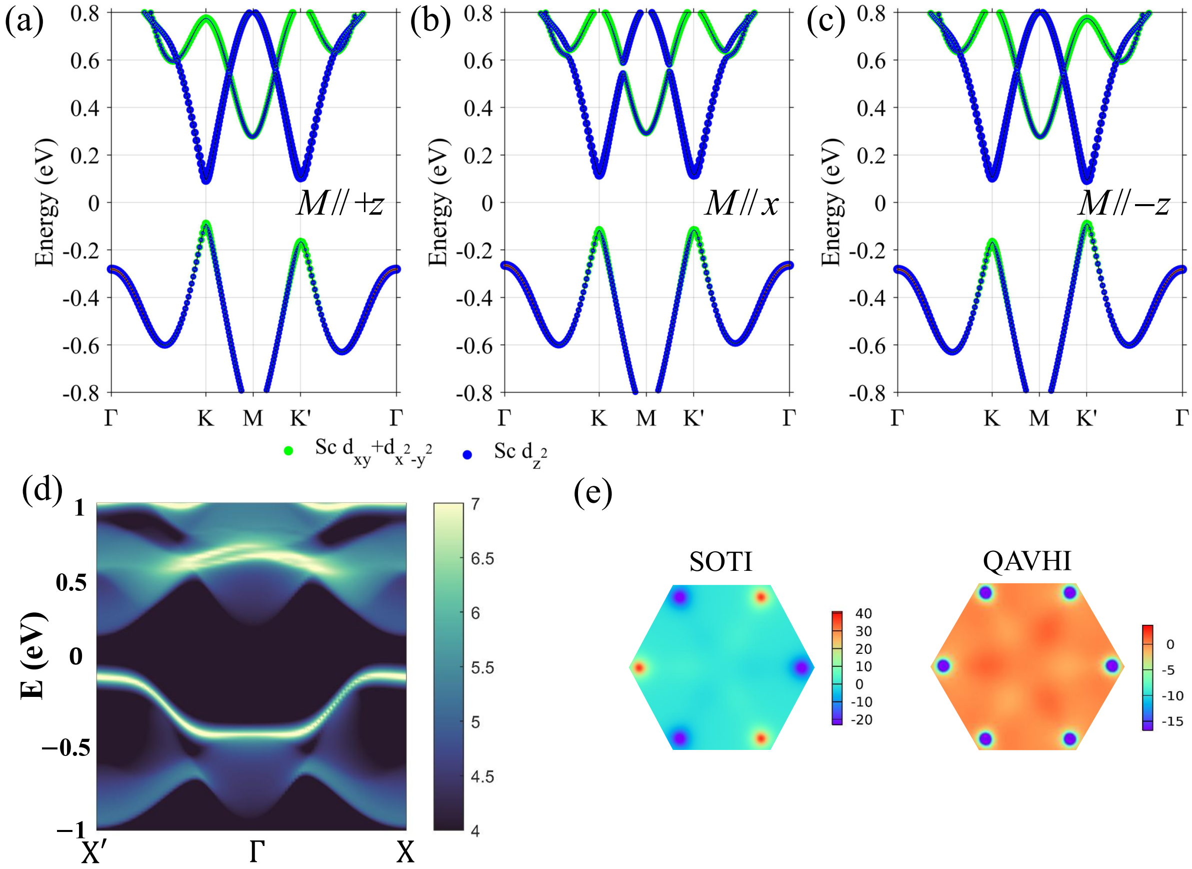


FIG. S4: (a-c) Projected energy band structures under three magnetic order directions. (d) Strain-free nanostrip surface band.(e) Berry curvature ascent maps of the first Brillouin zone of SOTI and QAVHI.

2D ScClI has a strong magnetic valley coupling effect, and the coupling strength depends on the magnitude of the magnetic moment projection in the Z direction, as shown in Fig. S4(a-c). When the magnetic moment is in in-plane magnetic order, the magnetic valley coupling is zero and valley polarization does not occur. And when the magnetism shifts from upward to downward, the valley polarization undergoes a responsive transition.

For the SOTI phase of ScClI, its intrinsically infinite nanoribbon surface band is shown in Fig. S4(d). Under the modulation of strain engineering, the energy band is reversed in the K-valley and accompanied by the change of Berry curvature, as shown in Fig. S4(e).

## IV. ANOMALOUS NERNST EFFECT

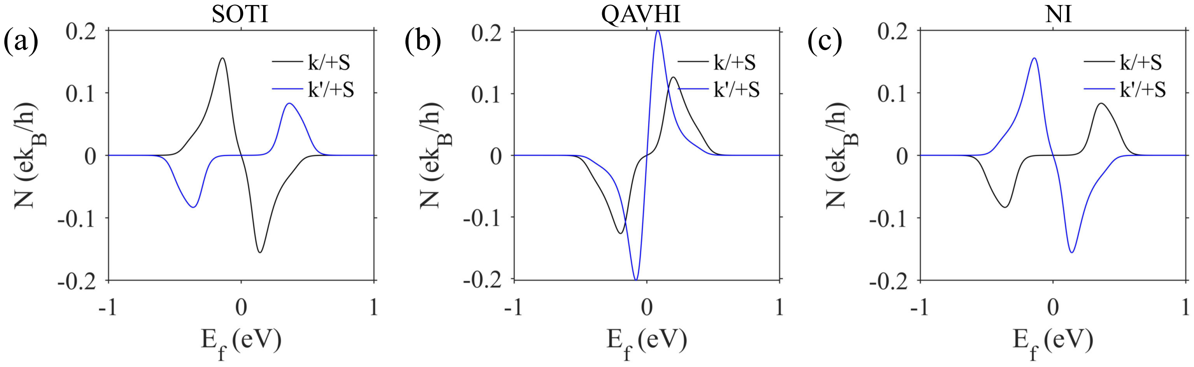


FIG. S5: The valley related anomalous Nernst conductivity of SOTI, QAVHI, and NI are characterized in (a, b, c), respectively

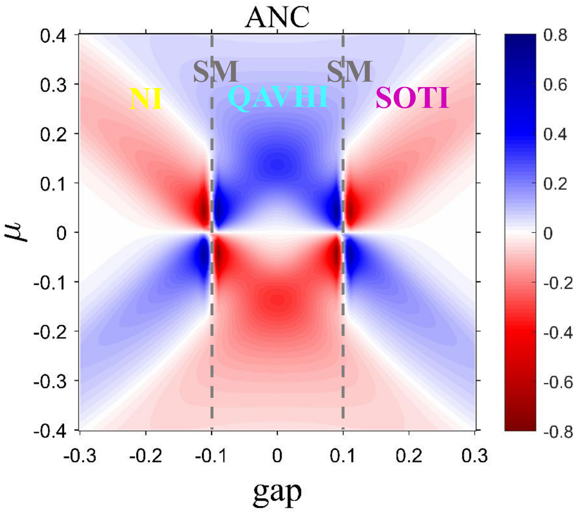


FIG. S6: ANC ascent charts on gap and $\mu$

Because of the valley polarization due to the intrinsic ferromagnetism of ScClI, the anomalous nernst conductance associated with the valleys has different properties. Figure S4 illustrates the valley-associated anomalous nernst conductance for three different insulators. Figure S6 illustrates the ascent diagram of ANC modulation with gap and mu. It can be seen that the charge flow ANC of NI and SOTI have the same characteristics, so ANC is not a good physical quantity to discriminate the higher-order topological phase.
